# Supplementary material for: EXPLORER: Exploration-guided Reasoning for Textual Reinforcement Learning
Source: arXiv:2403.10692 source file (2024-03-15)
Supplement: Supplementary file 1 [file appendix.tex]

% \section{Confidence Scoring Detail} \label{appx:conf_score}

% Confidence score of a learned rule is crucial as it projects the reliability of a rule. In our work, the rules are learned in two different ways - using ILP and generalizing them later with WordNet. So, the agent calculates the confidence score based on two separate components - (i) coverage of a rule while playing, and (ii) the distance between two nodes (entity and the hypernym) in the WordNet ontology. The coverage of a rule can be calculated by the number of times the rule gives a positive reward divided by the total number of times the rule has been used. Whereas the WordNet-based confidence gives a higher score to the parent of an entity than its grandparent and also the direct ILP learned rules get 1.0 (maximum score in this component). The cumulative maximum  score of the two components is 2.0 (1.0 from each component). Note that the \textit{neuro-symbolic rules} do not get the second component score as they do not possess any generalization (their maximum score is 1.0). Figure \ref{fig:gen_rule_conf} shows a snippet of a learned set of rules with different confidence scores. Rules (1) and (2) got the maximum score of 2 which means they were learned from the ILP and always got positive rewards when it was applied. Rules (3), (4), (5), and (6) got better to medium scores and we can clearly see why. For example, we normally put \textit{dairy products} to the \textit{fridge} or \textit{head-gears} to the \textit{hat-rack}. Rule (7) did not get a good score as it is a very generalized not-reliable rule saying - things that have a \textit{structure} goes to the \textit{fridge}. 
% \begin{figure}[t]
%     \centering
%     \includegraphics[scale = 1.0]{images/rules_conf.pdf}
%     \caption{Example of Rule's Confidence Scores (medium level games) }
%     \label{fig:gen_rule_conf}
% \end{figure}


% \section{Fallback Scenario} \label{appx:fallback}
% In EXPLORER, when the symbolic agent fails to provide a good action, the neural agent serves as a fallback. In other words, \ex accords priority to the symbolic actions based on the confidence scores. \ex fallbacks to the neural actions when either of the one following situations happens: (i) no policies for the given state because of early exploration stage or non-rewarded actions, or  
%  (ii) non-admissible symbolic actions has been generated due to rule generalization. 




% \begin{table*}[b]
%     \centering
%     \small
%     \begin{tabular}{|c|c|c|c|c|c|c|}
%     \hline
%     \multicolumn{1}{|l|}{\multirow{2}{*}{}} & \multicolumn{2}{c|}{\begin{tabular}[c]{@{}c@{}}Text-Only \\ (Neural)\end{tabular}} & \multicolumn{2}{c|}{\begin{tabular}[c]{@{}c@{}} GATA \\ (Neural)\end{tabular}} & \multicolumn{2}{c|}{\begin{tabular}[c]{@{}c@{}} EXPLORER-w/o-GEN \\ (Neuro-Symbolic) \end{tabular}} \\ \cline{2-7} 
%     \multicolumn{1}{|c|}{}                  & \multicolumn{1}{c|}{\#Steps}            & \multicolumn{1}{c|}{N. Score}      & \multicolumn{1}{c|}{\#Steps}            & \multicolumn{1}{c|}{N. Score}     & \multicolumn{1}{c|}{\#Steps}          & \multicolumn{1}{c|}{N. Score}          \\ \hline
%     Level-1 & 11.50 $\pm$ 1.26 & 0.93 $\pm$ 0.01 & 12.01 $\pm$ 0.84 & 0.72 $\pm$ 0.3 & \textbf{9.17 $\pm$ 3.28} & \textbf{0.96 $\pm$ 0.04} \\ 
%     Level-2 & 45.79 $\pm$ 1.56 & 0.35 $\pm$ 0.07 & 28.65 $\pm$ 1.28 & 0.23 $\pm$ 0.06 & \textbf{15.60 $\pm$ 3.74} & \textbf{0.58 $\pm$ 0.04} \\ 
%     Level-3 & 46.91 $\pm$ 1.51 & 0.25 $\pm$ 0.01 & 37.6 $\pm$ 1.17 & 0.18 $\pm$ 0.07 & \textbf{26.92 $\pm$ 2.74} & \textbf{0.34 $\pm$ 0.01} \\ 
%     Level-4 & 22.03 $\pm$ 0.19 & 0.76 $\pm$ 0.01 & 35.53 $\pm$ 2.5 & 0.34 $\pm$ 0.06 & \textbf{19.85 $\pm$ 2.12} & \textbf{0.85 $\pm$ 0.07}\\ \hline

%     \end{tabular}
%     \caption{ TW-Cooking domain --- Comparison Results (with Mean and SD) }
%     \label{tab:results_cooking_full}
% \end{table*}
% \section{Exhaustive vs IG based Generalization} \label{appx:exhaus_ig_gen}
% After doing extensive studies of \textit{exhaustive} vs. \textit{IG based} rule generalization, we found that in exhaustive generalization, the rules are lifted without considering the reliability of the generalized rules. By adding exceptions, the exception learning module takes care of it and tunes the low reliable rules to powerful rules that work with different other objects. Oppositely, for an object, due to the presence of the exceptional scenario (negative example) for a particular hypernym, the information gain becomes lower for that hypernym in comparison with others. So, IG-based generalization does not learn that rule. In another sense, the IG-based generalization only learns the best hypernyms and that is much more effective when the agent has seen many objects and their correct locations (more exploration). The \textit{easy} and \textit{medium} game results depict the same.
% Figure \ref{fig:gen_rule_example} shows two snippets of learned rules from the \textit{exhaustive generalization} and the \textit{IG-based generalization} for the entities whose location is \textit{shoe cabinet}. Both of the generalization methods learn almost the same set of rules, except the exhaustive one learns two more rules (rule no. 3 \& 5). The reason behind this is the comprehensive generalization with exception learning. So, in exhaustive generalization first, the rules are lifted with the hypernyms without considering the negative examples and later exception learner adds that negative example as an exception to fit all the examples with the learned rules. So, `scarf', which is a type of `covering' but does not go to a `shoe cabinet', learned as an exception (rule no. 5) to rule no. 3. In IG-based generalization, due to the presence of a negative example (the `scarf'), the information gain for `covering' goes down in comparison with the other hypernyms. This ends up in not learning the rule for `covering' in IG-based generalization.

%  \begin{figure}[t]
%     \centering
%     \includegraphics[scale = 1.0]{images/rules_example.drawio.pdf}
%     \caption{Generalized Rule Examples (medium level games)}
%     \label{fig:gen_rule_example}
% \end{figure}

% \section{TW-Cooking Full Result} \label{appx:twc-cooking-full-results}
% Table \ref{tab:results_cooking_full} demonstrates the comparison results with mean and standard deviation (SD).  

% \section{s(CASP) Engine} \label{appx:scasp}
%     s(CASP) \cite{scasp}  is a query-driven, goal-directed implementation of ASP that includes constraint solving over reals. Goal-directed execution of s(CASP) is indispensable for automating commonsense reasoning, as traditional grounding and SAT-solver based implementations of ASP may not be scalable. There are three major advantages of using the s(CASP) system: (i) s(CASP) does not ground the program, which makes our framework scalable, (ii) it only explores the parts of the knowledge base that are needed to answer a query, and (iii) it provides natural language justification  (proof tree) for an answer \cite{scasp_justification}.


% \section{EXPLORER Architecture}
% Figure~\ref{fig:hns_arch} illustrates the components of our neuro-symbolic architecture and shows an overview of the agent's decision-making process. 
%  \begin{figure}[t]
%     \centering
%     \includegraphics[scale = 0.45]{images/arch_diagram.pdf}
%     \caption{Overview of EXPLORER's decision-making at any given time step. The Hybrid Neuro-Symbolic architecture mainly consists of 5 modules - (a) \textcolor{Green}{Context Encoder} encodes the observation to dynamic context, (b) \textcolor{SkyBlue}{Action Encoder} encodes the admissible actions, (c) \textcolor{RedViolet!100}{Neural Action Selector} combines (a) and (b) with $\bigoplus$ operator, (d) \textcolor{blue}{Symbolic Action Selector} returns a set of candidate actions, and (e) \textcolor{BurntOrange}{Symbolic Rule Learner} uses ILP and WordNet-based rule generalization to generate symbolic rules.}
%     \label{fig:hns_arch}
% \end{figure}






% \section{TWC-Example} \label{appx:TWC_ex}
% Here are more details about the figure \ref{fig:game_example}, that we omitted because of the space constraint. In this section, we also show another detailed example as well.
% To generate action using the symbolic module, the agent first extracts the information about the entities from the observation and the inventory information. Then, this information is represented as ASP facts along with the hypernyms of the objects. Next, it runs the ASP solver - the s(CASP) engine to get a set of possible actions and select an action based on the confidence scores. The top-left section of figure \ref{fig:game_example} shows how a symbolic action that has been selected by matching the object (i.e., clean checked shirt) with the rule set (highlighted in the right). Here, the solver finds the location of the \textit{shirt} in \textit{wardrobe} as \textit{`clothing'} and \textit{`wearable'} are the hypernyms of the word - \textit{shirt}. So, whenever the agent does not find a symbolic action or fails to get a reward from the suggested symbolic action, then it moves to the neural agent to get an action (as a fallback). The bottom-left of figure \ref{fig:game_example} shows that the location of `sugar' is not covered by any rules, so the neural agent selects an action. Figure \ref{fig:game_neuro_symbolic_example} shows two different scenarios of the game - (a) symbolic agent works and neural fails, and (b) neural agent works and symbolic fails. This is how the symbolic and neural modules work in tandem.

% \begin{sidewaysfigure*}[ht!]
%     \centering
%     \includegraphics[scale = 1.3]{images/game_neuro_symbolic_example.pdf}
%     \caption{Two instances of TWC games, showing two different scenarios - (A) when symbolic agent works and neural agent fails, and (B) when symbolic agent fails and neural agent works }
%     \label{fig:game_neuro_symbolic_example}
% \end{sidewaysfigure*}


% \section{TW-Cooking Training graphs}
% Here is an example of training graphs for the easy games



% \cleardoublepage
% \section{Play Through} \label{appx:play-through}
% Here, we will provide a game play-through from the level - 4 games. We will provide two different agents' play one after the other for the same game.

%  %Text only Neural Agent (LSTM - A2C) 
% \noindent\fbox{%
%     \parbox{\textwidth}{%
%     \begin{center}
%         Text-Only Neural Agent (LSTM - A2C)  \\
%     \end{center}
        
%        \textbf{\underline{Step 1}}\\
%        \underline{\textit{Observation:}} \\
%        -= Corridor =- Well how about that, you are in the place we're calling the corridor. You start to take note of what's in the room. You don't like doors? Why not try going east, that entranceway is not blocked by one. There is an exit to the north. Don't worry, there is no door. There is an exit to the south.\\ 
%        \underline{\textit{Action:}} go east \\
%        \underline{\textit{Reward:}} 0 \\
%        \medskip

%        \textbf{\underline{Step 2}}\\
%        \underline{\textit{Observation:}} \\
%        -= Bedroom =- You've entered a bedroom.  You can make out a bed. But there isn't a thing on it.  You need an exit without a door? You should try going west.\\ 
%        \underline{\textit{Action:}} 
%        go west \\
%        \underline{\textit{Reward:}} 
%        0 \\
%        \medskip

%        \textbf{\underline{Step 3}}\\
%        \underline{\textit{Observation:}} \\
%        -= Corridor =- Well how about that, you are in the place we're calling the corridor. You start to take note of what's in the room.    You don't like doors? Why not try going east, that entranceway is not blocked by one. There is an exit to the north. Don't worry, there is no door. There is an exit to the south.  
%        \\ 
%        \underline{\textit{Action:}} 
%        go north \\
%        \underline{\textit{Reward:}} 
%        0 \\
%        \medskip

%        \textbf{\underline{Step 4}}\\
%        \underline{\textit{Observation:}} \\
%        -= Bathroom =- Well, here we are in a bathroom.  You scan the room, seeing a toilet. You wonder idly who left that here. The toilet is white. But the thing is empty, unfortunately.  You don't like doors? Why not try going south, that entranceway is not blocked by one.   
%        \\ 
%        \underline{\textit{Action:}} 
%        go south \\
%        \underline{\textit{Reward:}} 
%        0 \\
%        \medskip

%        \textbf{\underline{Step 5}}\\
%        \underline{\textit{Observation:}} \\
%        -= Corridor =- Well how about that, you are in the place we're calling the corridor. You start to take note of what's in the room.    You don't like doors? Why not try going east, that entranceway is not blocked by one. There is an exit to the north. Don't worry, there is no door. There is an exit to the south.
%        \\ 
%        \underline{\textit{Action:}} 
%        look \\
%        \underline{\textit{Reward:}} 
%        0 \\
%        \medskip
%     }
% }
% \clearpage

% \noindent\fbox{%
%     \parbox{\textwidth}{%
%        \textbf{\underline{Step 6}}\\
%        \underline{\textit{Observation:}} \\
%        -= Corridor =- Well how about that, you are in the place we're calling the corridor. You start to take note of what's in the room.    You don't like doors? Why not try going east, that entranceway is not blocked by one. There is an exit to the north. Don't worry, there is no door. There is an exit to the south.
%        \\ 
%        \underline{\textit{Action:}} 
%        go north \\
%        \underline{\textit{Reward:}} 
%        0 \\
%        \medskip

%        \textbf{\underline{Step 7}}\\
%        \underline{\textit{Observation:}} \\
%        -= Bathroom =- Well, here we are in a bathroom.  You scan the room, seeing a toilet. You wonder idly who left that here. The toilet is white. But the thing is empty, unfortunately.  You don't like doors? Why not try going south, that entranceway is not blocked by one. 
%        \\ 
%        \underline{\textit{Action:}} 
%        examine toilet \\
%        \underline{\textit{Reward:}} 
%        0 \\
%        \medskip

%        \textbf{\underline{Step 8}}\\
%        \underline{\textit{Observation:}} \\
%        The toilet is stable.
%        \\ 
%        \underline{\textit{Action:}} 
%        go south \\
%        \underline{\textit{Reward:}} 
%        0 \\
%        \medskip

%        \textbf{\underline{Step 9}}\\
%        \underline{\textit{Observation:}} \\
%          -= Corridor =- Well how about that, you are in the place we're calling the corridor. You start to take note of what's in the room.    You don't like doors? Why not try going east, that entranceway is not blocked by one. There is an exit to the north. Don't worry, there is no door. There is an exit to the south.
%        \\ 
%        \underline{\textit{Action:}} 
%        go south \\
%        \underline{\textit{Reward:}} 
%        0 \\
%        \medskip

%        \textbf{\underline{Step 10}}\\
%        \underline{\textit{Observation:}} \\
%        -= Livingroom =- You've just walked into a livingroom. I guess you better just go and list everything you see here.  Oh, great. Here's a sofa. The sofa is comfy. Unfortunately, there isn't a thing on it. Aw, and here you were, all excited for there to be things on it!  There is an exit to the east. Don't worry, there is no door. There is an exit to the north. Don't worry, there is no door.
%        \\ 
%        \underline{\textit{Action:}} 
%        examine sofa \\
%        \underline{\textit{Reward:}} 
%        0 \\
%        \medskip

%        \textbf{\underline{Step 11}}\\
%        \underline{\textit{Observation:}} \\
%        The sofa is durable.
%        \\ 
%        \underline{\textit{Action:}} 
%        go east \\
%        \underline{\textit{Reward:}} 
%        0 \\
%        \medskip
%     }
% }
% \clearpage
% \noindent\fbox{%
%     \parbox{\textwidth}{%    
%        \textbf{\underline{Step 12}}\\
%        \underline{\textit{Observation:}} \\
%        -= Kitchen =- You're now in the kitchen.  You can see a closed fridge close by. You see a closed oven in the corner. You can see a table! The table is massive. On the table you can see a cookbook. You can see a counter. The counter is vast. However, the counter, like an empty counter, has nothing on it. Oh! Why couldn't there just be stuff on it? You see a stove. But the thing is empty, unfortunately. You move on, clearly done caring about TextWorld.  There is a closed frosted-glass door leading east. You don't like doors? Why not try going west, that entranceway is not blocked by one. 
%        \\ 
%        \underline{\textit{Action:}} 
%        open fridge \\
%        \underline{\textit{Reward:}} 
%        0 \\
%        \medskip

%        \textbf{\underline{Step 13}}\\
%        \underline{\textit{Observation:}} \\
%        You open the fridge, revealing a sliced roasted white onion and a red onion.
%        \\ 
%        \underline{\textit{Action:}} 
%        take white onion from fridge \\
%        \underline{\textit{Reward:}} 
%        1 \\
%        \medskip

%        \textbf{\underline{Step 14}}\\
%        \underline{\textit{Observation:}} \\
%        You take the white onion from the fridge.   
       
%        Your score has just gone up by one point. 
%        \\ 
%        \underline{\textit{Action:}} 
%        prepare meal \\
%        \underline{\textit{Reward:}} 
%        1 \\
%        \medskip

%        \textbf{\underline{Step 15}}\\
%        \underline{\textit{Observation:}} \\
%         Adding the meal to your inventory.   
        
%         Your score has just gone up by one point.
%        \\ 
%        \underline{\textit{Action:}} 
%        eat meal \\
%        \underline{\textit{Reward:}} 
%        1 \\
%        \medskip

%        \textbf{\underline{Step 16}}\\
%        \underline{\textit{Observation:}} \\
%         You eat the meal. Not bad.  
        
%         Your score has just gone up by one point.
%        \\ 
%        \medskip

% Scored: 3 out of 3.

% *** The End ***  
       
%         }
% }

% \clearpage
% \noindent\fbox{%
%     \parbox{\textwidth}{%
%     \begin{center}
%        EXPLORER: A Neuro-Symbolic Agent  \\
%     \end{center}
        
%        \textbf{\underline{Step 1}}\\
%        \underline{\textit{Observation:}} \\
%        -= Corridor =- Well how about that, you are in the place we're calling the corridor. You start to take note of what's in the room. You don't like doors? Why not try going east, that entranceway is not blocked by one. There is an exit to the north. Don't worry, there is no door. There is an exit to the south.\\ 
%        \underline{\textit{Action:}} go south \\
%        \underline{\textit{Reward:}} 0 \\
%        \medskip

%        \textbf{\underline{Step 2}}\\
%        \underline{\textit{Observation:}} \\
%        -= Livingroom =- You've just walked into a livingroom. I guess you better just go and list everything you see here.  Oh, great. Here's a sofa. The sofa is comfy. Unfortunately, there isn't a thing on it. Aw, and here you were, all excited for there to be things on it!  There is an exit to the east. Don't worry, there is no door. There is an exit to the north. Don't worry, there is no door.\\ 
%        \underline{\textit{Action:}} 
%        go east \\
%        \underline{\textit{Reward:}} 
%        0 \\
%        \medskip

%        \textbf{\underline{Step 3}}\\
%        \underline{\textit{Observation:}} \\
%        -= Kitchen =- You're now in the kitchen.  You can see a closed fridge close by. You see a closed oven in the corner. You can see a table! The table is massive. On the table you can see a cookbook. You can see a counter. The counter is vast. However, the counter, like an empty counter, has nothing on it. Oh! Why couldn't there just be stuff on it? You see a stove. But the thing is empty, unfortunately. You move on, clearly done caring about TextWorld.  There is a closed frosted-glass door leading east. You don't like doors? Why not try going west, that entranceway is not blocked by one.   
%        \\ 
%        \underline{\textit{Action:}} 
%        examine cookbook \\
%        \underline{\textit{Reward:}} 
%        0 \\
%        \medskip

%        \textbf{\underline{Step 4}}\\
%        \underline{\textit{Observation:}} \\
%        You open the copy of "Cooking: A Modern Approach (3rd Ed.)" and start reading: \\ 
%        Recipe 1 --------- Gather all following ingredients and follow the directions to prepare this tasty meal.  \\
%        Ingredients:   white onion  \\Directions:   slice the white onion   roast the white onion   prepare meal   
%        \\ 
%        \underline{\textit{Action:}} 
%        open fridge \\
%        \underline{\textit{Reward:}} 
%        0 \\
%        \medskip

%        \textbf{\underline{Step 5}}\\
%        \underline{\textit{Observation:}} \\
%        You open the fridge, revealing a sliced roasted white onion and a red onion.
%        \\ 
%        \underline{\textit{Action:}} 
%        take white onion from fridge \\
%        \underline{\textit{Reward:}} 
%        1 \\
%        \medskip
%     }
% }


% \clearpage

% \noindent\fbox{%
%     \parbox{\textwidth}{%
    
%        \textbf{\underline{Step 6}}\\
%        \underline{\textit{Observation:}} \\
%        You take the white onion from the fridge.   
       
%        Your score has just gone up by one point. 
%        \\ 
%        \underline{\textit{Action:}} 
%        prepare meal \\
%        \underline{\textit{Reward:}} 
%        1 \\
%        \medskip

%        \textbf{\underline{Step 7}}\\
%        \underline{\textit{Observation:}} \\
%         Adding the meal to your inventory.   
        
%         Your score has just gone up by one point.
%        \\ 
%        \underline{\textit{Action:}} 
%        eat meal \\
%        \underline{\textit{Reward:}} 
%        1 \\
%        \medskip

%        \textbf{\underline{Step 8}}\\
%        \underline{\textit{Observation:}} \\
%         You eat the meal. Not bad.  
        
%         Your score has just gone up by one point.
%        \\ 
%        \medskip

% Scored: 3 out of 3.
 
% *** The End *** 
       
%         }
% }
